# Supplementary material for: FLAC: A Robust Failure-Aware Atomic Commit Protocol for Distributed Transactions
Source: arXiv:2302.04500 source file (2023-03-02)
Supplement: Supplementary file 1 [file appendix.tex]

\appendix

\section{Draft}

\phxsays{I am trying to explain the result of learning $\numRunNF$, and to see whether it is good to put it back to the paper.
I draft the description here first}

%ooibc: even if it s negative, need to give some results and explain why
% Noted

%\section{Learning $\alpha_{\mathsf{NF}}$}
%%% Local Variables:
%%% mode: latex
%%% TeX-master: "../main"
%%% End:

\phxedit{
[Technical Report.]

Here we give a detailed reason why {\prac} can shorten the time each participant to decide.
We only discuss 2PC because Easy Commit takes a longer time to decide on participants as shown in \cite{gupta2018easycommit}.
Let $t(x, y)$ to be the transmission time between $x, y$.
We can have all messages transmitted with the shortest path between $t(u, v)$ and $t(C^*, u) + t(C^*, v)$.
The time cost for a participant $u$ executed with {\prac} in \textit{fast path} to decide the result for transaction $T$ is $max\{ t(u, v) + t(C^*, v) | v \in {\nodesT} \}$.
Meanwhile, the time cost for a participant $u$ executed with 2PC to decide the result for transaction $T$ is
$ t(C^*, u) + 2 max\{ t(C^*, v) | v \in {\nodesT} \} = max\{ t(C^*, u) + 2t(C^*, v) | v \in {\nodesT} \} \ge max\{ t(u, v) + t(C^*, v) | v \in {\nodesT} \}.$
In all, {\prac} can always make participants stay undecided for a shorter time than 2PC in \textit{fast path}. Such an improvement in decide time is more significant when $max\{t(C^*, v) | v \in {\nodesT} \}$ is close to $max\{t(u, v) | v \in {\nodesT} \}$.
}
